# Supplementary material for: Reduced transition probabilities for the gamma decay of the 7.8 eV isomer in $^{229}$Th
Source: arXiv:1704.07919 source file (2017-06-11)
Supplement: Supplementary file 1 [file SupplMatLB15795.pdf]

# Reduced transition probabilities for the $\gamma$-decay of the 7.8 eV isomer in $^{229}$Th: Supplementary Material

N. Minkov[1,2] and A. Pálffy[2]

[1] *Institute of Nuclear Research and Nuclear Energy, Bulgarian Academy of Sciences, Tzarigrad Road 72, BG-1784 Sofia, Bulgaria*

[2] *Max-Planck-Institut für Kernphysik, Saupfercheckweg 1, D–69117 Heidelberg, Germany*

In the following we give in more detail factors and expressions which enter the analytical formalism presented in the main article text.

The centrifugal term in Eq. (2) of the Letter has the form:

$$\widetilde{X}(I^\pi, K_b) = \frac{1}{2}\Bigg[d_0 + I(I+1) - K_b^2 + (-1)^{I+\frac{1}{2}}\left(I+\frac{1}{2}\right) a_{\frac{1}{2}}^{(\pi\pi^b)}\delta_{K_b,\frac{1}{2}} - A \sum_{\substack{\nu\neq b \\ (K_\nu=\frac{1}{2},K_b\pm 1)}} \frac{\left[\widetilde{a}_{K_\nu K_b}^{(\pi\pi^b)}(I)\right]^2}{\epsilon_{\rm qp}^{K_\nu} - \epsilon_{\rm qp}^{K_b}}\Bigg], \tag{S1}$$

where $d_0$ determines the QO potential origin, the quantity $a_{1/2}^{(\pi,\pi^b)} = \pi\pi_b a_{\frac{1}{2}-\frac{1}{2}}^{(\pi^b)}$ represents the decoupling factor for the case $K_b = 1/2$ and $\widetilde{a}_{K_\nu K_b}^{(\pi,\pi^b)}$ represent the Coriolis mixing factors:

$$\widetilde{a}_{K_\nu K_b}^{(\pi,\pi^b)}(I) = \begin{cases} \sqrt{(I-K_b)(I+K_b+1)}\,a_{K_\nu K_b}^{(\pi^b)}\ , & K_\nu = K_b + 1\ , \\ \sqrt{(I+K_b)(I-K_b+1)}\,a_{K_b K_\nu}^{(\pi^b)}\ , & K_\nu = K_b - 1\ , \\ \pi\cdot\pi^b(-1)^{(I+\frac{1}{2})}(I+\frac{1}{2})a_{\frac{1}{2},-\frac{1}{2}}^{(\pi^b)}\ , & K_\nu = K_b = \frac{1}{2}\ , \end{cases} \tag{S2}$$

with

$$a_{K_\nu K_b}^{(\pi^b)} = \frac{P_{K_\nu K_b}^b}{N_{K_\nu}^{(\pi^b)} N_{K_b}^{(\pi^b)}} \langle \mathcal{F}_{K_\nu}^{(\pi^b)} | \hat{j}_+ | \mathcal{F}_{K_b}^{(\pi^b)} \rangle = \frac{P_{K_b K_\nu}^b}{N_{K_b}^{(\pi^b)} N_{K_{\nu'}}^{(\pi^b)}} \langle \mathcal{F}_{K_b}^{(\pi^b)} | \hat{j}_- | \mathcal{F}_{K_\nu}^{(\pi^b)} \rangle. \tag{S3}$$

The latter involve the matrix elements of the s.p. operators $\hat{j}_\pm = \hat{j}_x \pm i\hat{j}_y$ between the parity-projected components of the s.p. wave functions $\mathcal{F}_{K_b}^{(\pi^b)}$ of the band-head state and the admixing state $\mathcal{F}_{K_\nu}^{(\pi^b)}$, determined by DSM [21], where $\pi^b$ is the experimentally assigned parity of the band-head s.p. state. The quantity $N_K^{(\pi^b)} = \left[\left\langle \mathcal{F}_K^{(\pi^b)} \middle| \mathcal{F}_K^{(\pi^b)} \right\rangle\right]^{\frac{1}{2}}$ is a parity-projected normalization factor, whereas $P_{K_{\nu'} K_\nu}^b = U_{K_{\nu'}}^b U_{K_\nu}^b + V_{K_{\nu'}}^b V_{K_\nu}^b$ involves the BCS

occupation factors. The index $b$ corresponds to the blocked s.p. orbital on which the collective spectrum is built. Since the BCS procedure is performed separately for each band-head orbital (blocked) the overlap integrals and the matrix elements between states built on different band-head orbitals involve the average of both separate occupation factors $P^{bb'}_{K_{\nu'}K_{\nu}} = \frac{1}{2}\left(P^{b}_{K_{\nu'}K_{\nu}} + P^{b'}_{K_{\nu}K_{\nu'}}\right)$. The sum in (S1) runs over q.p. states with energies $\epsilon^{K_\nu}_{\text{qp}}$ above the Fermi level and $A$ is the Coriolis mixing strength defined in [24]. In our numerical calculations we consider ten mixing orbitals.

The Coriolis perturbed/mixed wave function for a QO spectrum built on a q.p. state with $K = K_b$ and parity $\pi^b$ is obtained in the form

$$\widetilde{\Psi}^{\pi,\pi^b}_{nkIMK_b} = \frac{1}{\widetilde{N}_{I\pi K_b}}\left[\Psi^{\pi,\pi^b}_{nkIMK_b} + A \sum_{\substack{\nu\neq b \\ (K_\nu = K_b\pm 1, \frac{1}{2})}} C^{I\pi}_{K_\nu K_b}\Psi^{\pi,\pi^b}_{nkIMK_\nu}\right], \tag{S4}$$

where the expansion coefficients are given by $C^{I\pi}_{K_\nu K_b} = \widetilde{a}^{(\pi\pi^b)}_{K_\nu K_b}(I)/(\epsilon^{K_\nu}_{\text{qp}} - \epsilon^{K_b}_{\text{qp}})$ and $\widetilde{N}^2_{I\pi K_b}$ is the normalization constant of the form

$$\begin{aligned}\widetilde{N}^2_{I\pi K_b} &= \left\langle \widetilde{\Psi}^{\pi,\pi^b}_{nkIMK_b} \middle| \widetilde{\Psi}^{\pi,\pi^b}_{nkIMK_b}\right\rangle \\ &= 1 + 2A \sum_{\substack{\nu\neq b \\ (K_\nu = K_b = \frac{1}{2})}} C^{I\pi}_{K_\nu K_b}\delta_{K_\nu K_b}\frac{P^b_{K_\nu K_b}}{N^{(\pi^b)}_{K_\nu}N^{(\pi^b)}_{K_b}}\left\langle \mathcal{F}_{K_\nu}{}^{(\pi^b)} \middle| \mathcal{F}_{K_b}{}^{(\pi^b)}\right\rangle \\ &+ A^2 \sum_{\substack{\nu_1\neq b \\ (K_{\nu_1} = K_b\pm 1, \frac{1}{2})}} \sum_{\substack{\nu_2\neq b \\ (K_{\nu_2} = K_b\pm 1, \frac{1}{2})}} C^{I\pi}_{K_{\nu_1}K_b}C^{I\pi}_{K_{\nu_2}K_b}\delta_{K_{\nu_1}K_{\nu_2}}\frac{P^b_{K_{\nu_1}K_{\nu_2}}}{N^{(\pi^b)}_{K_{\nu_1}}N^{(\pi^b)}_{K_{\nu_2}}}\left\langle \mathcal{F}_{K_{\nu_1}}{}^{(\pi^b)} \middle| \mathcal{F}_{K_{\nu_2}}{}^{(\pi^b)}\right\rangle .\end{aligned} \tag{S5}$$

The unperturbed QO core plus particle wave function in Eq. (S4) has the form [24]

$$\begin{aligned}\Psi^{\pi,\pi^b}_{nkIMK}(\eta,\phi,\theta) &= \frac{1}{N^{(\pi^b)}_K}\sqrt{\frac{2I+1}{16\pi^2}}\Phi^{\pi\cdot\pi^b}_{nkI}(\eta,\phi) \\ &\times \left[D^I_{M\,K}(\theta)\mathcal{F}^{(\pi^b)}_K + \pi\cdot\pi^b(-1)^{I+K}D^I_{M\,-K}(\theta)\mathcal{F}^{(\pi^b)}_{-K}\right],\end{aligned}$$

where $D^I_{M\,K}(\theta)$ are the rotation (Wigner) functions and $\Phi^{\pi\cdot\pi^b}_{nkI}(\eta,\phi)$ are the QO vibration functions obtained after solving the Schrödinger equation for the Hamiltonian (2) in ellipsoidal coordinates given by $\beta_2 = p\eta\cos\phi$ and $\beta_3 = q\eta\sin\phi$, with $p = \sqrt{d/d_2}$, $q = \sqrt{d/d_3}$, $d = (d_2 + d_3)/2$ and by assuming coherent quadrupole-octupole oscillations with a frequency $\omega = \sqrt{C_2/B_2} = \sqrt{C_3/B_3} \equiv \sqrt{C/B}$, as done in Refs. [19,20,27]. The function $\Phi^{\pi\cdot\pi^b}_{nkI}(\eta,\phi)$

involves Laguerre polynomials of the radial variable $\eta$ and cos (sin) functions of the angular variable $k\phi$, with $k$ = odd (even) integer for the even (odd) parity states of the core (see e.g. [27] for details).

For calculating the $B(E1)$, $B(E2)$ and (eventually) $B(E3)$ reduced probabilities for transitions between initial (i) and final (f) states given by Eq. (S4) and energies given by Eq. (3) in the Letter we use the operators and the matrix elements for the electric transitions in CQOM as given in Ref. [27], whereas for $B(M1)$ we take the M1 operator given in Ref. [25] [e.g. see Eq. (3.61) therein]. It appears that the expressions for both types ($T$), electric ($T = E$) and magnetic ($T = M$) transition with multipolarity $\lambda$ can be derived in a common form

$$
\begin{aligned}
&B(T\lambda;\pi^{b_i}I_i\pi_iK_i \to \pi^{b_f}I_f\pi_fK_f) = R^{T\lambda}\delta_{\pi^{b_f}\pi^{b_i}}\left[(1+\pi_f\pi_i(-1)^{\lambda\delta_{T,E}})/2\right]\\
&\times \frac{1}{\widetilde{N}^2_{I_f\pi_fK_f}\widetilde{N}^2_{I_i\pi_iK_i}}\Bigg[\delta_{K_fK_i}C^{I_fK_f}_{I_iK_i\lambda 0}\frac{P^{b_fb_i}_{K_fK_i}M^{\pi^{b_f}\pi^{b_i}}_{K_fK_i}}{N^{(\pi^{b_f})}_{K_f}N^{(\pi^{b_i})}_{K_i}}\\
&+ A\, C^{I_fK_f}_{I_iK_f\lambda 0}\sum_{\substack{\nu\neq i\\(K_\nu=K_i\pm 1,\frac{1}{2})}}\delta_{K_fK_\nu}C^{I_i\pi_i}_{K_\nu K_i}\frac{P^{b_f}_{K_fK_\nu}M^{\pi^{b_f}\pi^{b_i}}_{K_fK_\nu}}{N^{(\pi^{b_f})}_{K_f}N^{(\pi^{b_i})}_{K_\nu}}\\
&+ A\, C^{I_fK_i}_{I_iK_i\lambda 0}\sum_{\substack{\nu\neq f\\(K_\nu=K_f\pm 1,\frac{1}{2})}}\delta_{K_\nu K_i}C^{I_f\pi_f}_{K_\nu K_f}\frac{P^{b_i}_{K_\nu K_i}M^{\pi^{b_f}\pi^{b_i}}_{K_\nu K_i}}{N^{(\pi^{b_f})}_{K\nu}N^{(\pi^{b_i})}_{K_i}} \qquad \text{(S6)}\\
&+ A^2\sum_{\substack{\nu''\neq f\\(K_{\nu''}=K_f\pm 1,\frac{1}{2})}}\sum_{\substack{\nu'\neq i\\(K_{\nu'}=K_i\pm 1,\frac{1}{2})}}\delta_{K_{\nu''}K_{\nu'}}C^{I_fK_{\nu''}}_{I_iK_{\nu'}\lambda K_{\nu''}-K_{\nu'}}C^{I_f\pi_f}_{K_{\nu''}K_f}C^{I_i\pi_i}_{K_{\nu'}K_i}\frac{P^{b_fb_i}_{K_{\nu''}K_{\nu'}}M^{\pi^{b_f}\pi^{b_i}}_{K_{\nu''}K_{\nu'}}}{N^{(\pi^{b_f})}_{K_{\nu''}}N^{(\pi^{b_i})}_{K_{\nu'}}}\Bigg]^2,
\end{aligned}
$$

where $R^{T\lambda=E\lambda} = \frac{2\lambda+1}{4\pi(4-3\delta_{\lambda,1})}R^2_\lambda(\pi^{b_i}n_ik_iI_i \to \pi^{b_f}n_fk_fI_f)$ involves integrals on the radial and angular variables in CQOM (see Eqs. (35)–(41) and Appendices B and C in Ref. [27]) and $R^{T1=M1} = \frac{3}{4\pi}\mu_N^2$ involves the nuclear magneton; $M^{\pi^{b_f}\pi^{b_i}}_{K_fK_i} = \langle\mathcal{F}^{(\pi^{b_f})}_{K_f}|\mathcal{F}^{(\pi^{b_i})}_{K_i}\rangle$ for T=E and $M^{\pi^{b_f}\pi^{b_i}}_{K_fK_i} = \left[(g_l-g_R)K_i\delta_{K_fK_i}\langle\mathcal{F}^{(\pi^{b_f})}_{K_f}|\mathcal{F}^{(\pi^{b_i})}_{K_i}\rangle + (g_s-g_l)\langle\mathcal{F}^{(\pi^{b_f})}_{K_f}|\hat{s}_z|\mathcal{F}^{(\pi^{b_i})}_{K_i}\rangle\right]$, for T=M. Here $g_R = Z/A_{\rm mass}$ is the rotation gyromagnetic factor, $\hat{s}_z$ is the $z$-component of the spin operator, $g_l = 0\,(1)$ for neutrons (protons) is the orbital gyromagnetic factor, whereas the spin gyromagnetic factor is $g_s = 0.6\ g_s^{\rm free}$ with $g_s^{\rm free} = -3.826\,(5.586)$ for neutrons (protons). The notation $C^{I_fK_f}_{I_iK_i\lambda 0}$ denotes the Clebsch-Gordan coefficient.

We note that the term on the second line of Eq. (S6) above corresponds to the unperturbed part of the wave function. Note that the overlap integral $\langle\mathcal{F}^{(\pi^{b_f})}_{K_f}|\mathcal{F}^{(\pi^{b_i})}_{K_i}\rangle$ may have nonzero

value only if the $K$ values of the initial and final band-head orbitals $b_i$ and $b_f$ are equal, $K_f = K_i$, though the orbitals still can be different ($b_f \neq b_i$). The terms on the third and fourth lines of (S6) provide a first order $K$- mixing effect and practically contribute with non-zero values only in the cases $K_{i/f} = K_\nu = 1/2$, i.e. when a $K_{i/f} = 1/2$ band-head state is mixed with another $K_\nu = 1/2$ state present in the considered range of admixing orbitals above the Fermi level. The last term in (S6) involves a second order mixing effect which may connect states with $\Delta K = 1, 2$. The overlap integral $\langle \mathcal{F}^{(\pi^{b_f})}_{K_{\nu''}} | \mathcal{F}^{(\pi^{b_i})}_{K_{\nu'}} \rangle$ is nonzero only for $K_{\nu''} = K_{\nu'}$ (not necessarily =1/2), whereas the product $C^{I_f \pi_f}_{K_{\nu''} K_f} C^{I_i \pi_i}_{K_{\nu'} K_i}$ allows different combinations of $|K_i - K_f| \leq 2$ which provide respective non-zero contribution of the Coriolis mixing to the transition probability. Therefore, this term is very important to get a non-zero transition probability between states with different $K$-values.

In Table S1 below the parameters of the calculations made for several combinations of $k^{(-)}_{\rm yr}$ and $k^{(-)}_{\rm ex}$ values are given together with the respectively predicted $B(E2)$ and $B(M1)$ values for the $3/2^+_{\rm ex} \to 5/2^+_{\rm yr}$ transition.

TABLE S1: Theoretical $E_{\rm ex}(\frac{3}{2}^+)$ isomer energy (in keV) and predicted $B(E2)$ and $B(M1)$ values (in W.u.) for the $3/2^+_{\rm ex} \to 5/2^+_{\rm yr}$ transition in $^{229}$Th obtained for different sets of model parameters $\omega$ [MeV/$\hbar$], $b$ [$\hbar^{-2}$], $d_0$ [$\hbar^2$], $c$ and $p$ (dimensionless) and $A$ [keV]. $k^{(-)}_{\rm yr}$ and $k^{(-)}_{\rm ex}$ correspond to negative-parity sequences. For the BCS pairing constants we have used the parameter values $g_0 = 18.805$ and $g_1 = 7.389$ (see Eq. (4) in Ref. [22]), tuned in order to obtain a suitably small q.p. energy for the $3/2^+$ isomeric state. The rms$_{\rm yr}$, rms$_{\rm ex}$ and rms$_{\rm tot}$ deviations for the yrast, excited and total energy spectrum are given in keV.

| $\omega$ | $b$ | $d_0$ | $c$ | $p$ | $A$ | $k^{(-)}_{\rm yr}$ | $k^{(-)}_{\rm ex}$ | rms$_{\rm yr}$ | rms$_{\rm ex}$ | rms$_{\rm tot}$ | $E_{\rm ex}(\frac{3}{2}^+)$ | $B(E2)$ | $B(M1)$ |
|---|---|---|---|---|---|---|---|---|---|---|---|---|---|
| 0.2039 | 0.28 | 18 | 79 | 1.0 | 0.158 | 2 | 2 | 39.9 | 26.0 | 34 | 0.4263 | 27.04 | 0.0076 |
| 0.2361 | 0.28 | 33 | 89 | 1.0 | 0.141 | 2 | 2 | 41.2 | 26.4 | 35 | 0.0078 | 23.05 | 0.0061 |
| 0.0912 | 2.39 | 49 | 245 | 1.0 | 0.152 | 4 | 6 | 37.6 | 15.8 | 29 | 0.3556 | 25.80 | 0.0071 |
| 0.0635 | 4.51 | 45 | 321 | 1.0 | 0.144 | 6 | 8 | 36.4 | 12.4 | 28 | 0.0725 | 22.86 | 0.0063 |
| 0.0563 | 7.34 | 66 | 473 | 1.0 | 0.138 | 8 | 10 | 38.3 | 11.9 | 29 | $10^{-9}$ | 21.31 | 0.0058 |
